# Supplementary material for: Elle: Inferring Isolation Anomalies from Experimental Observations
Source: arXiv:2003.10554 source file (2020-03-23)
Supplement: Supplementary file 1 [file appendix.tex]

Proof of lemma \ref{traceable->x_max-trace-all-committed}.

\begin{proof}
Assume some committed version $x_i$ is not in the trace of $x_{max}$. Clearly, $x_i \neq x_{max}$. Since $\ll$ is total, $x_i \ll x_{max}$. By axiom \ref{version-order->version-graph}, there must exist a path from $x_i \xrightarrow{} x_{max}$, and since $x$ is traceable, there must be a path from $x_{init}$ to $x_i$. This implies that there are two distinct paths from $x_{init}$ to $x_{max}$: one, the trace of $x_{max}$, and the other, passing through $x_i$. However, traceable objects, by definition, have only one path from $x_{init}$ to any $x_i$: a contradiction.
\end{proof}

Proof of lemma \ref{list-append-is-traceable}.

\begin{proof}
By the definition of list append objects, a write to $x$ is of the form $w(x_i = [e_1, \ldots, e_n], a) \xrightarrow{} (x'_i = [e_1, \ldots, e_n, a], nil)$.

The initial object $x_{init} = []$ has a single trace: $[x_{init}]$, since no append operation can result in an empty list.

Now consider an version other than $x_{init}$: $x_j = [b_1 \ldots b_{m-1}, b_m]$. What edges in $v_x$ lead to $x_j$? By our definition of $w$ for list append, any inbound edges on $x_j$ must be of the form $w(x_i = [a_1 \ldots a_{n-1}], a_n) \xrightarrow{} ([a_1 \ldots a_{n-1}, a_n], nil)$, for all $x_i$. Since this write results in $x_j$, we know that $n = m$, and $a_1 = b_1$, $a_2 = b_2$, and so on, up to $a_n = b_m$. This implies there is exactly one $x_i$ ($[a_1 \ldots a_{n-1}$]) and argument $a_n$ ($b_m$) for any $x_j \neq x_{init}$.

Since $x_{init}$ has one trace, and every version other than $x_{init}$ has exactly one preceding version and write connecting them, every $x_j$ has exactly one trace.
\end{proof}
