# Supplementary material for: Elle: Inferring Isolation Anomalies from Experimental Observations
Source: arXiv:2003.10554 source file (2020-03-23)
Supplement: Supplementary file 2 [file appendix_peter.tex]

In this section we provide proofs of the lemmata defined in the main body of the paper.  Along the way, we define a number of auxiliary lemmata and axioms.

\section{Preliminaries}

\subsection{Definition of $x_{max}$}

\section{Theory of Mind}

\subsection{Recoverability}

\paragraph{Prefix Lemma}

\subsection{Dirty Reads}

In this section we provide proofs of the lemmata defined in Section~\ref{sec:dirty}.
